# Supplementary material for: Non conforming vector finite elements for H(curl) intersected with H(div)
Source: arXiv:1101.0587 ancillary file (2011-08-24)
Supplement: Supplementary file 1 [file NonConformingFormalCheck.pdf]

The following is a basis BaseHarm of the vector space of harmonic polynomials of degree 4.

```
In[1]:= BaseHarm = {y^4 - 6 * y^2 * z^2 + z^4,
  x * y^3 - 3 * x * y * z^2, x^2 * y^2 - x^2 * z^2 - y^2 * z^2 + z^4 / 3,
  x^3 * y - 3 * x * y * z^2, x^4 - 6 * x^2 * z^2 + z^4, y^3 * z - y * z^3,
  x * y^2 * z - (x * z^3) / 3, x^2 * y * z - (y * z^3) / 3, x^3 * z - x * z^3};
```

Indeed its elements are harmonic,

```
In[2]:= D[BaseHarm, {x, 2}] + D[BaseHarm, {y, 2}] + D[BaseHarm, {z, 2}]
```

```
Out[2]:= {0, 0, 0, 0, 0, 0, 0, 0, 0}
```

and its cardinality and rank are equal to the dimension of this vector space.

```
In[3]:= {Length[BaseHarm],
  MatrixRank[Join@@Join@@Table[{i, j, k}, {i, 0, 4}, {j, 0, 4}, {k, 0, 4}] /.
  (Append[#, {x_, y_, z_} → 0] & /@
  (CoefficientRules[#, {x, y, z}] & /@ BaseHarm))]}]
```

```
Out[3]:= {9, 9}
```

We also introduce a basis BaseP2 of the collection of polynomials of degree <= 2,

```
In[4]:= BaseP2 = {1, x, y, z, x^2, y^2, z^2, x y, y z, z x};
```

and a basis BaseVec of the space of polynomial vector fields P23 defined in the paper.

```
In[5]:= Zeroes = Array[0 &, 10];
```

```
Grad[P_] := {D[P, x], D[P, y], D[P, z]};
```

```
BaseVec = Join[
  Transpose[{BaseP2, Zeroes, Zeroes}],
  Transpose[{Zeroes, BaseP2, Zeroes}],
  Transpose[{Zeroes, Zeroes, BaseP2}],
  Grad /@ BaseHarm
];
```

The following computes the moments of order 0 of the elements of BaseVec on the tetrahedron T0.

```
In[8]:= MT0 = Transpose[Integrate[BaseVec, {x, 0, 1}, {y, 0, 1 - x}, {z, 0, 1 - x - y}]];
```

We now compute the moments of order <= 1 on the faces {x=0}, {y=0}, {z=0} and {x+y+z=1} of T0.

```
In[9]:= BaseVecX = BaseVec /. x -> 0;
BaseVecY = BaseVec /. y -> 0;
BaseVecZ = BaseVec /. z -> 0;
BaseVecXYZ = BaseVec /. z -> (1 - x - y);
```

```
MTX = Join[
  Transpose[Integrate[BaseVecX, {y, 0, 1}, {z, 0, 1 - y}]],
  Transpose[Integrate[y BaseVecX, {y, 0, 1}, {z, 0, 1 - y}]],
  Transpose[Integrate[z BaseVecX, {y, 0, 1}, {z, 0, 1 - y}]]
];
MTY = Join[
  Transpose[Integrate[BaseVecY, {x, 0, 1}, {z, 0, 1 - x}]],
  Transpose[Integrate[x BaseVecY, {x, 0, 1}, {z, 0, 1 - x}]],
  Transpose[Integrate[z BaseVecY, {x, 0, 1}, {z, 0, 1 - x}]]
];
MTZ = Join[
  Transpose[Integrate[BaseVecZ, {x, 0, 1}, {y, 0, 1 - x}]],
  Transpose[Integrate[x BaseVecZ, {x, 0, 1}, {y, 0, 1 - x}]],
  Transpose[Integrate[y BaseVecZ, {x, 0, 1}, {y, 0, 1 - x}]]
];
MTXYZ = Join[
  Transpose[Integrate[BaseVecXYZ, {x, 0, 1}, {y, 0, 1 - x}]],
  Transpose[Integrate[x BaseVecXYZ, {x, 0, 1}, {y, 0, 1 - x}]],
  Transpose[Integrate[y BaseVecXYZ, {x, 0, 1}, {y, 0, 1 - x}]]
];
```

The following matrix M gathers the above linear functionals. Their common null space is the same as the common null space of the linear functionals N23 defined in the paper.

```
In[17]:= M = Join[MT0, MTX, MTY, MTZ, MTXYZ];
```

As expected M is a 39x39 square matrix,

```
In[18]:= {Length[M], Length[M[[1]]]}
```

```
Out[18]= {39, 39}
```

which it is rank deficient.

```
In[19]:= MatrixRank[M]
```

```
Out[19]= 38
```

This matrix has a one dimensional nullspace,

```
In[20]:= nsp = NullSpace[M]
```

```
Out[20]= {{1/10, 0, -3/5, -3/5, 1, -1/2, -1/2, -1, 8, -1, 1/10, -3/5, 0, -3/5, -1/2, 1, -1/2, -1, -1, 8,
1/10, -3/5, -3/5, 0, -1/2, -1/2, 1, 8, -1, -1, -1/2, 1, 3/2, 1, -1/2, 1, -6, -6, 1}}
```

a representative of which is given in the paper.

```
In[21]:= P = 3 * x + 10 * x^3 - 15 * x^4 + 3 * y - 18 * x * y - 15 * x^2 * y + 30 * x^3 * y - 15 * x * y^2 +
45 * x^2 * y^2 + 10 * y^3 + 30 * x * y^3 - 15 * y^4 + 3 * z - 18 * x * z - 15 * x^2 * z +
30 * x^3 * z - 18 * y * z + 240 * x * y * z - 180 * x^2 * y * z - 15 * y^2 * z -
180 * x * y^2 * z + 30 * y^3 * z - 15 * x * z^2 + 45 * x^2 * z^2 - 15 * y * z^2 -
180 * x * y * z^2 + 45 * y^2 * z^2 + 10 * z^3 + 30 * x * z^3 + 30 * y * z^3 - 15 * z^4;
```

```
Simplify[30 nsp[[1]].BaseVec == Grad[P]]
```

```
Out[22]= True
```
